# Supplementary material for: Quantum Natural Gradient with Efficient Backtracking Line Search
Source: arXiv:2211.00615 source file (2022-11-01)
Supplement: Supplementary file 1 [file mole_ham_appendix.tex]

This appendix reviews molecular Hamiltonian construction and evaluation, in light of computational chemistry via Hartree Fock theory and/or Second Quantization, in this particular order: (1) electronic structure theory, (2) molecular orbitals and Slater determinants, (3) Hartree-Fock approximation, (4) fermionic ladder operators, and (5) qubit operators.
Sections \ref{esp} - \ref{hft} prescribes the Hartree Fock approach via molecular orbitals, Fock operators, and a variational methodology, whereas sections \ref{second_quant} - \ref{qubit_ham} prescribes the Second Quantization approach via fermionic ladders followed by the Jordan-Wigner transformation to qubit operators.

\subsubsection{Electronic Structure Problem}
\label{esp}
As a prelude to the former approach, molecules and materials are to be approximated as many-electron systems. To consider a many-electron system, geometric configuration of the nuclei and electrons are to be approximated, ({\color{red}[Figure ?]}) followed by the Born-Oppenheimer approximation of the molecular Hamiltonian operator, 
\begin{equation}
\label{BOA}
    \hat{H} =\sum_{i=1}^{N}\frac{1}{2} \nabla_i^2 - \sum_{i=1}^{N}\sum_{A=1}^{M}\frac{Z_A}{r_{iA}} + \sum_{i=1}^{N}\sum_{j>i}^{N}\frac{1}{r_{ij}}.
\end{equation}
Above, $\nabla_i^2$ is the second-order Laplacian of the $i^{th}$-electron, $Z_A$ is the atomic number for the $A^{th}$-nucleus, $r_{iA}$ is the Euclidean distance between the $i^{th}$-electron and $A^{th}$-nucleus, and $r_{ij}$ is the Euclidean distance between the $i^{th}$-electron and $j^{th}$-electron. \ref{BOA} corresponds to the system's total electronic energy and energy spectrum - deduced from the time-independent electronic Schrodinger equation,
\begin{equation*}
    \hat{H}\ket{\Psi} = E\ket{\Psi}.
\end{equation*}
In liaison, fermionic particles (i.e. - electrons) are indistinguishable. Hence, $\ket{\Psi}$, an electronic eigenstate (per energy spectrum, E) of the N-electrons system, must be a superposition of all possible configurations, which is $N!$ in total, 
\begin{equation}
\label{WF}
    \ket{\Psi} = \frac{1}{\sqrt{N!}}\sum_{\sigma_i}A_i\ket{\Psi_{\sigma_i}}.
\end{equation}
$\{\sigma_i\}$ are the various spatial permutations of electron configurations and $\{\ket{\Psi_{\sigma_i}}\}$ are the electronic wavefunctions per permutation $\sigma_i$. In addition, each permutation must be symmetric to each other, up to a global phase factor of $e^{i\phi}$, where the exchange of any two electrons in a state $\Psi_{\sigma_k}$ are described via permutation operators, P$_{ij}$, as
\begin{equation}
\label{permutation}
\begin{split}
    P_{ij}\ket{\Psi_{\sigma_k}} = P_{ij}\ket{\Psi_1(x_1)...\Psi_i(x_i)...\Psi_j(x_j)...\Psi_N(x_N)} \\
    = e^{i\phi}\ket{\Psi_1(x_1)...\Psi_i(x_j)...\Psi_j(x_i)...\Psi_N(x_N)}.
\end{split}
\end{equation}
$x_i$ is electron $i$, whereas $\Psi_i$ is defined as an orbital (further described in \ref{orbitals}); hence, in \ref{permutation}, electron $i$ is exchanged with electron $j$ from orbital $i$ to orbital $j$. 

In totality, given $P_{ij}$ per exchange,
\begin{equation}
\label{WF2}
    \ket{\Psi} = \frac{1}{\sqrt{N!}}\sum_{\sigma_i}e^{i\phi(\sigma_i)}\ket{\Psi_{\sigma_i}},
\end{equation}
where $A_i$=$e^{i\phi(\sigma_i)}$ from \ref{WF}. And, by deduction, measurement of the probability density of states $\ket{\Psi_1(x_1)...\Psi_i(x_i)...\Psi_j(x_j)...\Psi_N(x_N)}$ and $\ket{\Psi_1(x_1)...\Psi_i(x_j)...\Psi_j(x_i)...\Psi_N(x_N)}$, where the latter exchanges electrons between $\Psi_i$ and $\Psi_j$, are indistinguishable, as shown below,
\begin{equation*}
\begin{split}
    \|e^{i\phi}\ket{\Psi_1(x_1)...\Psi_i(x_j)...\Psi_j(x_i)...\Psi_N(x_N)}\|^2 \\
    = \bra{\Psi_1(x_1)...\Psi_i(x_j)...\Psi_j(x_i)...\Psi_N(x_N)}e^{i^{*}\Phi}e^{i\Phi}\ket{\Psi_1(x_1)...\Psi_i(x_j)...\Psi_j(x_i)...\Psi_N(x_N)} \\
    = \bra{\Psi_1(x_1)...\Psi_i(x_i)...\Psi_j(x_j)...\Psi_N(x_N)}\ket{\Psi_1(x_1)...\Psi_i(x_i)...\Psi_j(x_j)...\Psi_N(x_N)} \\
    = \|\ket{\Psi_1(x_1)...\Psi_i(x_i)...\Psi_j(x_j)...\Psi_N(x_N)}\|^2,
\end{split}
\end{equation*}
given that
\begin{equation*}
    \ket{\Psi_1(x_1)...\Psi_i(x_i)...\Psi_j(x_j)...\Psi_N(x_N)} = e^{i\Phi}\ket{\Psi_1(x_1)...\Psi_i(x_i)...\Psi_j(x_j)...\Psi_N(x_N)}
\end{equation*}
via required symmetry up to the global phase factor. Note, a double permutation of the same two electrons, in a state $\Psi_{\sigma_k}$, restricts the contributing phase factor to
\begin{equation*}
    e^{i\phi}e^{i\phi} = e^{2i\phi} = 1,
\end{equation*}
to reproduce the initial state $\Psi_{\sigma_k}$. Hence, the above is only true if $\phi$ = 0 or an integer multiple of $\pi$. 

The above restriction therefore restricts $e^{i\phi}$ to +1 (for equivalence class $\phi$ = $\{0\}$) and -1
(for equivalence class $\phi$ = $\{\pi\}$), where the latter is the associated class for fermionic eigenstates. The above restriction applied to the permutation operator on electronic states formulates the Antisymmetry principle. Hence, the phase factor in \ref{WF2} are simply +1 or -1, with respect to there being even or odd electron exchanges, respectively,
\begin{equation}
\label{WF3}
    \ket{\Psi} = \frac{1}{\sqrt{N!}}\sum_{\sigma_i}(-1)^{\Gamma(\sigma_i)}\ket{\Psi_{\sigma_i}},
\end{equation}
where $\Gamma(\sigma_i)$ is the number of electron exchanges in permutation $\sigma_i$. \ref{WF3} is mathematically prescribed as the Slater determinant, where 
\begin{equation}
\label{slater}
\ket{\Psi} = \frac{1}{\sqrt{N!}} det
\begin{pmatrix}
\Psi_{1}(x_1) & \cdots & \Psi_{N}(x_1) \\
\vdots  & \ddots & \vdots  \\
\Psi_{1}(x_N) & \cdots & \Psi_{N}(x_N)
\end{pmatrix}.
\end{equation}
Furthermore, given the above exchange symmetry, for a 2-electron system in particular, 
\begin{equation}
\label{twoX}
    \ket{\Psi} = \ket{\Psi_i(x_1)\Psi_j(x_2)} - \ket{\Psi_i(x_2)\Psi_j(x_1)},
\end{equation}
where
\begin{equation*}
\begin{split}
    P_{12}\ket{\Psi_i(x_1)\Psi_j(x_2)} = e^{i\pi}\ket{\Psi_i(x_2)\Psi_j(x_1)} \\
    = -\ket{\Psi_i(x_2)\Psi_j(x_1)},
\end{split}
\end{equation*}
if $i=j$,
% \begin{equation}
%     \ket{\Psi_1(x_1)} = \ket{\Psi_2},
% \end{equation}
then, by \ref{twoX},
\begin{equation*}
    \ket{\Psi} = 0,
\end{equation*}
which describes the mathematical impossibility of two electrons occupying the same state simultaneously. Thus, as a by-product of the Antisymmetry principle, the Pauli exclusion principle, where no two electrons may occupy the same state, is deduced.

Last, subject to a mean-field approximation per electron, a prescription of Hartree-Fock approximation, the approximate electronic energy of the system, given the electronic Slater determinant \ref{slater}, is prescribed as
\begin{equation}  
E_{HF} = -\sum_{i=1}^{N}\bra{\Psi_{i}}\frac{1}{2} \nabla^2\ket{\Psi_{i}} - \sum_{i=1}^{N}\bra{\Psi_{i}}\sum_{A=1}^{M}\frac{Z_A}{r_{iA}}\ket{\Psi_{i}}  + \sum_{i=1}^{N}\sum_{j>i}^{N}(\bra{\Psi_{i}\Psi_{j}}\ket{\Psi_{i}\Psi_{j}} - \bra{\Psi_{i}\Psi_{j}}\ket{\Psi_{j}\Psi_{i}}), \end{equation}
where the third and fourth terms are the two-electron Coulomb repulsion and exchange energies, respectively.
\subsubsection{Orbitals}
\label{orbitals}
Now, a prescription of the electronic wavefunctions, \ref{WF3}, of many-electron systems is provisioned here. Electronic wavefunctions are prescribed as molecular orbitals, where each molecular orbital is a linear combination of atomic orbital (AO) basis functions,
\begin{equation}
     \Psi_{m}^{\sigma}(r) = \sum_{\mu}^K C_{\mu m}^\sigma\Phi_{\mu}(r).
\end{equation}
\(\sigma \in\{\alpha, \beta\}\) is the $\frac{1}{2}$ and -$\frac{1}{2}$ spins of the molecular orbital, respectively, $\Phi_{\mu}(r)$ are the atomic orbital basis functions (w.r.t. spatial distance $r$ of an electron) and C$_{\mu m}^\sigma$ are the expansion coefficients of AO. By deduction, the electronic wavefunction density of the system is prescribed as \begin{equation}  \begin{split}  
    \rho(r) = 2\sum_{i}^{N/2}\Psi_{i}^{\sigma*}(r)\Psi_{i}^{\sigma}(r) \\  = 2\sum_{i}^{N/2}(\sum_{\mu=1}^K C_{\mu i}^{\sigma*}\Phi_{\mu}^{*}(r))(\sum_{\nu=1}^K C_{\nu i}^{\sigma}\Phi_{\nu}(r)) \\  = 2\sum_{\mu\nu}(\sum_{i=1}^{N/2} C_{\mu i}^{\sigma*}C_{\nu i}^{\sigma})\Phi_{\mu}^{*}(r)\Phi_{\nu}(r) \\  = 2\sum_{\mu\nu} P_{\mu\nu}^{\sigma}\Phi_{\mu}^{*}(r)\Phi_{\nu}(r),  
\end{split}  \end{equation}
where,
\begin{equation} 
    P_{\mu\nu}^{\sigma} = \sum_{i=1}^{N/2} C_{\mu i}^{*\sigma}C_{\nu i}^{\sigma}.
\end{equation}
Thus, 
\begin{equation}
    P_{\mu\nu} = P_{\mu\nu}^{\alpha} + P_{\mu\nu}^{\beta}.
\end{equation}
Henceforth, by contraction with the electronic wavefunction density tensor, the Hartree-Fock energy is computed as 
\begin{equation}  
    E_{HF} = \sum_{\mu\nu}P_{\mu\nu}h_{\mu\nu} + \frac{1}{2}\sum_{\mu\nu\kappa\lambda}P_{\mu\nu}P_{\kappa\lambda}(\mu\nu|\kappa\lambda) - \frac{a}{2}\sum_{\mu\nu\kappa\lambda}[P_{\mu\kappa}^{\alpha}P_{\nu\lambda}^{\alpha} + P_{\mu\kappa}^{\beta}P_{\nu\lambda}^{\beta}](\mu\nu|\kappa\lambda).
\end{equation}
$h_{\mu\nu}$ is the Hamiltonian-core, composed of one-electron kinetic energy integral operators, $T_{\mu\nu}$, and electron-nuclear potential integral energy operators, $V_{\mu\nu}$, pre-computed over the atomic orbital basis functions as,
\begin{equation}
    h_{\mu\nu} = T_{\mu\nu} + V_{\mu\nu}.
\end{equation}
Above,
\begin{equation}
    T_{\mu\nu} = -\int dr\ \Phi_{\mu}^*(r)(\frac{\nabla^2}{2})\Phi_{\nu}(r)
\end{equation}
and
\begin{equation}
    V_{\mu\nu} = -\int dr\  \Phi_{\mu}^*(r)(\sum_{A=1}^{M}\frac{Z_A}{r - R_A})\Phi_q(r).
\end{equation}
In tandem, $(\mu\nu|\kappa\lambda)$ is the two-electron repulsion integral operator, pre-computed over the atomic orbital basis functions as
\begin{equation}
    (\mu\nu|\kappa\lambda) = \int dr_1 \int dr_2\ \frac{\Phi_{\mu}^*(r_1)\Phi_{\nu}^*(r_2)\Phi_{\kappa}(r_2)\Phi_{\lambda}(r_1)}{|r_1 - r_2|}.
\end{equation}

\subsubsection{Hartree-Fock Theory}
\label{hft}
In liaison, an approximation method for computing optimal electronic wavefunctions for a system is deduced from the Variational Principle postulate. 

This derivation is the Hartree-Fock approximation, in particular, for restricted, closed-shell molecular systems, where $\alpha$ and $\beta$ molecular orbitals share the same atomic spatial orbitals:
\begin{equation*}
    P_{\mu\nu}^\alpha = P_{\mu\nu}^\beta = \frac{1}{2}P_{\mu\nu} = \sum_{i=1}^{N/2}C_{\mu i}C_{\nu i}.
\end{equation*}
Hence, under orthonormality constraint requirement prescribed to an optimal molecular orbital set, the expansion coefficients, $\{C_{\mu m}\}$, are optimized to obtain a stationary point of the Hartree-Fock energy via the Lagrangian,
\begin{equation}  
    L_{HF} = E_{HF} - \sum_{\mu\nu}\epsilon_{\mu\nu}[\bra{\mu}\ket{\nu} - \delta_{\mu\nu}],
\end{equation}
where
\begin{equation}
    \ket{\nu} = \Phi_{\nu}(r),
\end{equation}
\begin{equation}
    \delta_{\mu\nu} =
    \begin{cases}
      1, & \text{if}\ \mu=\nu \\
      0, & \text{otherwise}
    \end{cases}
\end{equation}
and $\epsilon_{\mu\nu}$ is a scale factor per orbital pair. In liaison, a stationary point is sought, w.r.t. \(C_{\mu m}\):
\begin{equation} 
    \frac{\partial L_{HF}}{\partial C_{\mu m}} = 0.
\end{equation}
Through further algebraic deduction, a generalized eigenvalue
problem is deduced,
\begin{equation}  
    FC = SCE,  
\end{equation}
where $C$ is the molecular orbitals non-orthonormalized expansion coefficient matrix, $S$ is the overlap matrix of the non-orthogonal basis function set, where
\begin{equation}
    S_{\mu\nu} = \int dr\ \Phi_{\mu}(r)\Phi_{\nu}(r),
\end{equation}
$F$ is the Fock operator, where
\begin{equation}  
\label{fock_op}
    F_{\mu\nu} = h_{\mu\nu} + \sum_{\kappa\lambda}[2(\mu\nu|\kappa\lambda) - (\mu\kappa|\nu\lambda)]P_{\lambda\kappa},
\end{equation}
and $E$ is the orbital energy diagonal matrix. 
% The eigenvalue problem above is non-linear; the Fock matrix depends on its eigenvectors through the density matrix. 
The above approximation is to be computed with an iterative protocol, the Roothan-Hall self consistent equation, as prescribed below:
\begin{itemize}
\tightlist
\item[i.]
  Compute the initial guess density
\item[ii.] 
  Start the Roothaan-Hall
  self-consistent iterations
\item[iii.]
  Run until a convergence criterion is met or
  until a set maximum number of iterations is met
\item[iv.]
  Use the norm of the difference between two successive density
  matrices, \[ || P^{[i+1]} - P^{[i]} || \] as the convergence criterion
\item[v.]
  At each iteration, form the Coulomb matrix, \(J\), using contraction
  of the density matrix and the pre-computed electron-repulsion integral tensor:
  \[ J_{\mu\nu}^{[i]} = \sum_{\kappa\lambda} (\mu\nu|\kappa\lambda)P_{\lambda\kappa}^{[i]} \]
\item[vi.]
  At each iteration, form the exchange, \(K\), using contraction of the
  density matrix and the pre-computed electron-repulsion integral tensor:
  \[ K_{\mu\nu}^{[i]} = \sum_{\kappa\lambda} (\mu\kappa|\nu\lambda)P_{\lambda\kappa}^{[i]} \]
\item[vii.]
  Energy per epoch is computed as
  \[ E^{[i]} = tr(h + F^{[i]})P^{[i]} + E_{NN}\]
  where $E_{NN}$ is the nuclear-nuclear repulsion energy tensor. 
\end{itemize}
Using NumPy, a Python-based package that provides methods for matrix multiplications, tensor
contractions, decompositions, and linear solvers, the above technique is provided programmatically [{\color{red} Should we upload a python script to a website? Or provide full program below at end of document?}].

\subsubsection{Second Quantization}
\label{second_quant}
Nonetheless, a computationally compressed approach is achieved via second quantization of electronic Schrodinger equation, in which antisymmetry of fermionic systems are transferred from Slater determinants of electronic molecular orbitals to fermionic operators. In tandem, the electronic states are captured via occupation number states,
\begin{equation}
    \ket{n_1, ... , n_K}.
\end{equation}
where,
\begin{equation}
    n_j =
    \begin{cases}
      1, & \text{if}\ \Psi_j  \text{is occupied by an electron} \\
      0, & \text{otherwise}
    \end{cases}.
\end{equation}
Hence, the electronic state is transformed from linear combination of Slater determinants to superposition of state represented via occupation numbers.

Now, the fermionic operators $a_k$ and $a_k^{\dag}$ must satisfy anticommutation relations:
\begin{equation}
    {a_j, a_k^{\dag}} = \delta_{jk}
\end{equation}
and
\begin{equation}
    {a_j, a_k} = {a_j^{\dag}, a_k^{\dag}} = 0,
\end{equation}
where their actions on the occupation number states are prescribed as below,
\begin{equation}
    a_j\ket{n_1, ... , n_K} = \del_{1,n_p}(-1)^{N_j}\ket{n_1, ..., n_j \oplus 1, ..., n_K},
\end{equation}
and
\begin{equation}
    a_j^{\dag}\ket{n_1, ... , n_K} = \del_{0,n_p}(-1)^{N_j}\ket{n_1, ..., n_j \oplus 1, ... , n_K}.
\end{equation}
$N_j = \sum_{i=1}^k n_i$ and $\oplus$ is modulo 2 operation on $n_j$. Thus, the exchange symmetry is encoded in the phase factor $(-1)^{N_k}$, as applied via the action of the fermionic operator.

Note that the optimized molecular orbital (OMO) orthogonalized set from Hartree Fock approximation may be provisioned as a warm-start orbital set to the inner-product formulations of the one-electron and two-electron integrals in the second-quantized fermionic Hamiltonian,
\begin{equation}
    \hat{H} = \sum_{pq} h_{pq}a_p^{\dagger}a_q + \frac{1}{2}\sum_{pqrs} h_{pqrs} a_p^{\dagger}a_q^{\dagger}a_ra_s
\end{equation}
where 
\begin{equation}
    \begin{split}
        \hat{h}_{pq} = \int dr\ \Psi_p^*(r)(-\frac{\nabla^2}{2} - \sum_{A=1}^{M}\frac{Z_A}{r - R_A})\Psi_q(r) \\
        = \int dr\ \sum_{\mu=1}^{k}c_{\mu}\Phi_{\mu}(r)(-\frac{\nabla^2}{2} - \sum_{A=1}^{M}\frac{Z_A}{r - R_A})\sum_{\nu=1}^{k}c_{\nu}\Phi_{\nu}(r)
    \end{split}
\end{equation}
and
\begin{equation}
    \hat{h}_{pqrs} = \int dr_1 \int dr_2\ \frac{\Psi_p^*(r_1)\Psi_q^*(r_2)\Psi_r(r_2)\Psi_s(r_1)}{|r_1 - r_2|}.
\end{equation}
By further algebraic deduction,
\begin{equation}
    \hat{h}_{pq} = \sum_{\mu\nu} C_{p\mu}h_{\mu\nu}C_{\nu q}
\end{equation}
and
\begin{equation}
    \hat{h}_{pqrs} = \sum_{\mu\nu\rho\sigma} C_{p\mu}C_{q\nu}h_{\mu\nu\rho\sigma}C_{\rho r}C_{\sigma s},
\end{equation}
where \(h_{\mu\nu}\) and \(h_{\mu\nu\rho\sigma}\) are the Hamiltonian-core and electron-repulsion tensor pre-computed for the Hartree-Fock operator, during Hartree-Fock approximation.

\subsubsection{Qubit Hamiltonian}
\label{qubit_ham}
However, execution of quantum simulation requires qubit-based operators. Hence, the derived second quantized Hamiltonian must be further transformed, where it maintains the fermionic exchange symmetries. This is achieved through the Jordan-Wigner transformation, as prescribed below:
\begin{itemize}
    \item[1] A state $\ket{n_1, ... , n_M}$ in the occupation number representation on $M$ spin-orbitals can be directly mapped to a state $\ket{n_1}\ket{n_2}$ ··· $\ket{n_M}$ on $M$ qubits, where the state of the $i^{th}$ qubit is $\ket{1}$ if the corresponding spin-orbital is occupied, and $\ket{0}$ otherwise.
    \item[2] Fermionic ladder operators are transformed as
    \begin{equation}
        a_p = \frac{1}{2}Z_0\cross...\cross Z_{p-1}(X_p + iY_p)
    \end{equation}
    \begin{equation}
        a_p^{\dag} = \frac{1}{2}Z_0\cross...\cross Z_{p-1}(X_p - iY_p)
    \end{equation}
    where $X$, $Y$, $Z$ are Pauli matrices.
    \item[3] The resulting Hamiltonian is
    \begin{equation}
        H = \sum_i k_i P_i
    \end{equation}
    where $P_i$ is a Pauli matrix ($X$, $Y$, $Z$), including $I$.
\end{itemize}
For H$_2$, using the STO-3G basis referenced in the paper, this procedure produces the Hamiltonian presented in the paper [{\color{red} Make sure reference the additional technique to reduce the Hamiltonian size from 4 to 2 qubits}],
\begin{equation}
    H_{\mathrm{H}_2} = \alpha_0 I_1 I_2 + \alpha_1 Z_1I_2 + \alpha_2 I_1Z_2 + \alpha_3 Z_1Z_2 + \alpha_4 Y_1Y_2 + \alpha_5 X_1X_2.
\end{equation}
